# Supplementary material for: Graph-Structured Speculative Decoding
Source: arXiv:2407.16207 source file (2024-07-23)
Supplement: Supplementary file 1 [file appendix_full.tex]

\begin{table}[h]
\begin{center}
\setlength{\tabcolsep}{1.2mm}{
\scalebox{0.8}{\begin{tabular}{lllll}
\toprule
Methods & 65B & 30B & 13B & 7B \\
\midrule
\textsc{Regular ICL} & 59.82 & 55.18 & 47.79 & 49.72 \\
\textsc{Rd} & 63.66 & 59.91 & 49.68 & 49.34 \\
\textsc{RdSca} & 75.76 & 69.32 & 53.03 & 50.92 \\
\midrule
\textit{with demonstration retrieval} \\
\textsc{Regular ICL} &  74.75 & 65.62 & 58.00 & 56.88 \\
\textsc{Rd} &  77.13 & 73.63 & 56.38 & 59.25 \\
\textsc{RdSca} &  87.38 & 82.13 & 68.88 & 64.63 \\
\bottomrule
\end{tabular}}}
\end{center}
\caption{Full evaluation results on SST-2}
\vspace{-1mm}
\end{table}

\begin{table}[h]
\begin{center}
\setlength{\tabcolsep}{1.2mm}{
\scalebox{0.8}{\begin{tabular}{lllll}
\toprule
Methods & 65B & 30B & 13B & 7B \\
\midrule
\textsc{Regular ICL} &  76.79 & 58.15 & 44.98 & 50.67 \\
\textsc{Rd} &  76.12 & 56.49 & 42.94 & 48.34 \\
\textsc{RdSca} &  76.90 & 56.17 & 46.97 & 50.66 \\
\midrule
\textit{with demonstration retrieval} \\
\textsc{Regular ICL} &  78.12 & 64.73 & 45.54 & 57.59 \\
\textsc{Rd} &  79.72 & 60.38 & 49.06 & 59.91 \\
\textsc{RdSca} &  79.72 & 60.38 & 52.83 & 57.08 \\
\bottomrule
\end{tabular}}}
\end{center}
\caption{Full evaluation results on CB}
\vspace{-1mm}
\end{table}

\begin{table}[h]
\begin{center}
\setlength{\tabcolsep}{1.2mm}{
\scalebox{0.8}{\begin{tabular}{lllll}
\toprule
Methods & 65B & 30B & 13B & 7B \\
\midrule
\textsc{Regular ICL} &  53.67 & 49.13 & 61.50 & 59.62 \\
\textsc{Rd} &  53.20 & 53.37 & 62.54 & 57.96 \\
\textsc{RdSca} &  59.68 & 53.44 & 60.05 & 57.23 \\
\midrule
\textit{with demonstration retrieval} \\
\textsc{Regular ICL} &  60.17 & 53.85 & 67.94 & 63.47 \\
\textsc{Rd} &  61.79 & 62.95 & 70.38 & 64.20 \\
\textsc{RdSca} &  64.87 & 61.54 & 66.79 & 64.36\\
\bottomrule
\end{tabular}}}
\end{center}
\caption{Full evaluation results on QQP}
\vspace{-1mm}
\end{table}

\begin{table}[h]
\begin{center}
\setlength{\tabcolsep}{1.2mm}{
\scalebox{0.8}{\begin{tabular}{lllll}
\toprule
Methods & 65B & 30B & 13B & 7B \\
\midrule
\textsc{Regular ICL} &  59.38 & 53.45 & 47.84 & 46.56 \\
\textsc{Rd} &  58.27 & 52.28 & 47.77 & 47.63 \\
\textsc{RdSca} &  60.51 & 54.49 & 45.33 & 47.29 \\
\midrule
\textit{with demonstration retrieval} \\
\textsc{Regular ICL} &  63.21 & 60.90 & 51.79 & 52.56 \\
\textsc{Rd} &  62.03 & 65.67 & 51.66 & 53.14 \\
\textsc{RdSca} &  64.43 & 66.15 & 51.27 & 52.98 \\
\bottomrule
\end{tabular}}}
\end{center}
\caption{Full evaluation results on QNLI}
\vspace{-1mm}
\end{table}

\begin{table}[h]
\begin{center}
\setlength{\tabcolsep}{1.2mm}{
\scalebox{0.8}{\begin{tabular}{lllll}
\toprule
Methods & 65B & 30B & 13B & 7B \\
\midrule
\textsc{Regular ICL} &  36.97 & 36.33 & 29.69 & 28.19 \\
\textsc{Rd} &  37.86 & 36.49 & 30.31 & 27.64 \\
\textsc{RdSca} &  43.85 & 40.09 & 31.12 & 30.89 \\
\midrule
\textit{with demonstration retrieval} \\
\textsc{Regular ICL} &  70.75 & 70.38 & 67.12 & 67.50 \\
\textsc{Rd} &  74.63 & 76.12 & 72.00 & 74.12 \\
\textsc{RdSca} &  75.13 & 76.25 & 70.12 & 70.75 \\
\bottomrule
\end{tabular}}}
\end{center}
\caption{Full evaluation results on AG-News}
\vspace{-1mm}
\end{table}

\begin{table}[h]
\begin{center}
\setlength{\tabcolsep}{1.2mm}{
\scalebox{0.8}{\begin{tabular}{lllll}
\toprule
Methods & 65B & 30B & 13B & 7B \\
\midrule
\textsc{Regular ICL} &  72.36 & 63.99 & 55.4 & 53.76 \\
\textsc{Rd} &  72.0 & 65.56 & 55.4 & 55.6 \\
\textsc{RdSca} &  73.07 & 65.8 & 57.07 & 53.95 \\
\midrule
\textit{with demonstration retrieval} \\
\textsc{Regular ICL} &  72.25 & 63.12 & 56.75 & 52.75 \\
\textsc{Rd} &  72.39 & 65.27 & 55.7 & 54.66 \\
\textsc{RdSca} &  74.07 & 65.92 & 56.74 & 53.23 \\
\bottomrule
\end{tabular}}}
\end{center}
\caption{Full evaluation results on RTE}
\vspace{-1mm}
\end{table}
